# Supplementary material for: Directional Multivariate Ranking
Source: arXiv:2006.09978 source file (2020-06-09)
Supplement: Supplementary file 1 [file supplement.tex]

\onecolumn
\section*{Supplementary Material}
\subsection*{Derivation of Eq.~\ref{eq:mulvarrank_ll}}
%placeholder
\begin{flalign}
\label{eq:eq13}
    \mathcal{L}(\Theta) &= \prod\limits_{(u,i,j)\in S}\int_{\xi}^{\infty} p(\bm D_{uij} = \gamma\cdot\bm d_{uij}|\Theta) d\gamma &\\\nonumber
    &= \prod\limits_{(u,i,j)\in S}\int_{\xi}^{\infty}\mathcal{N}(\gamma\cdot\bm d_{uij} |\, [U_u*(V_i-V_j)]W^T, \bm\Sigma_{uij}) d\gamma &\\\nonumber
    &= \prod\limits_{(u,i,j)\in S}\frac{1}{\sqrt{(2\pi)^K|\bm\Sigma_{uij}|}}\int_{\xi}^{\infty}  exp\big(-\frac{1}{2}(\gamma\cdot\bm d_{uij}-[U_u*(V_i-V_j)]W^T)\bm\Sigma_{uij}^{-1}(\gamma\cdot\bm d_{uij}-[U_u*(V_i-V_j)]W^T)^T\big) d\gamma &\nonumber
\end{flalign}
%placeholder
\begin{flalign*}
&Let \; \hat{\bm d}_{u,i,j} = \big(U_u*(V_i-V_j)\big)W^T;\;
A = \bm d_{uij}\bm\Sigma_{uij}^{-1}\bm d_{uij}^T,\; B = \bm d_{uij}\bm\Sigma_{uij}^{-1}\hat{\bm d}_{uij}^T,\; C = \hat{\bm d}_{uij}\bm\Sigma_{uij}^{-1}\hat{\bm d}_{uij}^T &
\end{flalign*}
%placeholder
\begin{flalign}
\label{eq:eq14}
    \Rightarrow &\int_{\xi}^{\infty}exp\big(-\frac{1}{2}(\gamma\cdot\bm d_{uij}-\hat{\bm d}_{u,i,j})\bm\Sigma_{uij}^{-1}(\gamma\cdot\bm d_{uij}-\hat{\bm d}_{u,i,j})^T\big) d\gamma &\\\nonumber
    =\;& exp(-\frac{1}{2}C)\cdot\int_{\xi}^{\infty} exp\big(-\frac{1}{2}(\gamma^2A - 2\gamma B)\big) d\gamma & \\\nonumber
    =\;& exp(-\frac{1}{2}C)\cdot\int_{\xi}^{\infty} exp\big(-\frac{1}{2}A(\gamma - \frac{B}{A})^2 + \frac{B^2}{2A}\big) d\gamma & \\\nonumber
    =\;& exp(\frac{B^2}{2A}-\frac{1}{2}C)\cdot\int_{\xi}^{\infty} exp\big(-\frac{1}{2}A(\gamma - \frac{B}{A})^2\big) d\gamma &
\end{flalign}
%placeholder
\begin{flalign*}
&\because \int_{a}^{b}exp(-x^2)dx = \frac{\sqrt\pi}{2}\big(erf(b)-erf(a)\big)& 
\end{flalign*}
%placeholder
\begin{flalign}
\label{eq:eq15}
    \Rightarrow &\int_{\xi}^{\infty}exp\big(-\frac{1}{2}A(\gamma - \frac{B}{A})^2\big) d\gamma 
    =\;\frac{\sqrt\pi}{2}\sqrt{\frac{2}{A}}erf\big(\sqrt{\frac{A}{2}}(\gamma-\frac{B}{A})\big)\Big|_\xi^\infty
    =\;\sqrt\frac{\pi}{2A}\Big(1 - erf\big(\sqrt{\frac{A}{2}}(\xi-\frac{B}{A})\big)\Big)& \\\nonumber
\end{flalign}
Substitute Eq.~\ref{eq:eq15} to Eq.~\ref{eq:eq14}, and the result of Eq.~\ref{eq:eq14} to Eq.~\ref{eq:eq13}, we have:
\begin{flalign}
\label{eq:eq16}
    \mathcal{L}(\Theta) &= \prod\limits_{(u,i,j)\in S}\int_{\xi}^{\infty} p(\bm D_{uij} = \gamma\cdot\bm d_{uij}|\Theta) d\gamma &\\\nonumber
    &= \prod\limits_{(u,i,j)\in S}\int_{\xi}^{\infty}\mathcal{N}(\gamma\cdot\bm d_{uij} |\, [U_u*(V_i-V_j)]W^T, \bm\Sigma_{uij}) d\gamma &\\\nonumber
    &= \prod\limits_{(u,i,j)\in S}\frac{1}{\sqrt{(2\pi)^K|\bm\Sigma_{uij}|}}exp\big(-\frac{1}{2}(C-\frac{B^2}{A})\big)\cdot\sqrt\frac{\pi}{2A}\Big(1 - erf\big(\sqrt{\frac{A}{2}}(\xi-\frac{B}{A})\big)\Big) &\nonumber
\end{flalign}
\clearpage

\subsection*{Gradients for Eq.~\ref{eq:mulvarrank_obj}}
We denote the Eq.~\ref{eq:mulvarrank_obj} as \textit{DMR}, and provides the gradients $\frac{\partial DMR}{\partial\Theta}$ with respect to all parameters.\\
\textbf{Gradients for $\bm U, \bm V, \bm W$:}\\
\begin{flalign}
\label{eq:eq17}
    &\frac{\partial DMR}{\partial\hat{\bm d}_{u,i,j}} = -\frac{1}{2}(\bm\Sigma_{uij}^{-1}+\bm\Sigma_{uij}^{-T})\hat{\bm d}_{u,i,j} + \frac{(\bm d_{u,i,j}\bm\Sigma_{uij}^{-1}\hat{\bm d}_{u,i,j}^T)(\bm d_{u,i,j}\bm\Sigma_{uij}^{-1})}{\bm d_{u,i,j}\bm\Sigma_{uij}^{-1}\bm d_{u,i,j}^T} + \frac{1}{1-erf(Z)}\cdot\frac{2}{\sqrt{\pi}}e^{-Z^2}\cdot\frac{\bm d_{u,i,j}\bm\Sigma_{uij}^{-1}}{\sqrt{2\bm d_{u,i,j}\bm\Sigma_{uij}^{-1}\bm d_{u,i,j}^T}}&
\end{flalign}
where $Z=\sqrt{\frac{\pi}{2A}}(\xi-\frac{B}{A})$. As $\hat{\bm d}_{u,i,j} = \big(U_u*(V_i-V_j)\big)W^T$, with the chain rule, we have:
\begin{flalign}
\label{eq:eq18}
    &\frac{\partial DMR}{\partial\bm U_u} = \frac{\partial DMR}{\partial\hat{\bm d}_{u,i,j}} \big((\bm V_i - \bm V_j)*\bm W\big) \\\nonumber
    &\frac{\partial DMR}{\partial\bm V_i} = \frac{\partial DMR}{\partial\hat{\bm d}_{u,i,j}} \big(\bm U_u*\bm W\big)  \\\nonumber
    &\frac{\partial DMR}{\partial\bm V_j} = -\frac{\partial DMR}{\partial\hat{\bm d}_{u,i,j}} \big(\bm U_u*\bm W\big)  \\\nonumber
    &\frac{\partial DMR}{\partial\bm W} = (\frac{\partial DMR}{\partial\hat{\bm d}_{u,i,j}})^T \big(\bm U_u*(\bm V_i - \bm V_j)\big)  \\\nonumber
\end{flalign}
When the Hadmard product is applied to $\bm W$, it broadcasts to each row of $\bm W$.\\
\\
\textbf{Gradients for $\bm\Sigma_{uij} $:}\\
\begin{flalign}
\label{eq:eq19}
    \frac{\partial DMR}{\partial\bm\Sigma_{uij}} =& -\frac{1}{2}\bm\Sigma_{uij}^{-T} + \frac{1}{2}(\bm\Sigma_{uij}^{-T}\hat{\bm d}_{u,i,j}\hat{\bm d}_{u,i,j}^T\bm\Sigma_{uij}^{-T}) &\\\nonumber
    &+\frac{1}{2A^2}\big[2AB(\bm\Sigma_{uij}^{-T}\bm d_{u,i,j}\hat{\bm d}_{u,i,j}^T\bm\Sigma_{uij}^{-T}) + B^2(\bm\Sigma_{uij}^{-T}\bm d_{u,i,j}\bm d_{u,i,j}^T\bm\Sigma_{uij}^{-T}) \big] &\\\nonumber
    &+\frac{\bm\Sigma_{uij}^{-T}\bm d_{u,i,j}\bm d_{u,i,j}^T\bm\Sigma_{uij}^{-T}}{2A} - \frac{1}{1-erf(Z)}(\frac{2}{\sqrt{\pi}}e^{-Z^2})\cdot\frac{\partial Z}{\partial \bm\Sigma_{uij}} &\\\nonumber
    \frac{\partial Z}{\partial\bm\Sigma_{uij}} =& -\frac{\xi}{2\sqrt{2A}}(\bm\Sigma_{uij}^{-T}\bm d_{u,i,j}\bm d_{u,i,j}^T\bm\Sigma_{uij}^{-T}) + \frac{1}{2A}\Big[\sqrt{2A}(\bm\Sigma_{uij}^{-T}\bm d_{u,i,j}\hat{\bm d}_{u,i,j}^T\bm\Sigma_{uij}^{-T}) - \frac{B}{2\sqrt{2A}}(\bm\Sigma_{uij}^{-T}\bm d_{u,i,j}\bm d_{u,i,j}^T\bm\Sigma_{uij}^{-T})\Big]
\end{flalign}
